# Supplementary material for: Agentic LLM reasoning in pediatric diabetes outcome prediction from multimodal medical records
Source: arXiv:2610.40379 source file (2026-10-29)
Supplement: Supplementary file 1 [file supp_xref.tex]

\makeatletter
\newlabel{stab:outcome_prevalence}{{1}{10}{}{}{}}
\newlabel{stab:cohort_composition}{{2}{10}{}{}{}}
\newlabel{stab:feature_availability}{{3}{11}{}{}{}}
\newlabel{stab:pooled_stats}{{4}{11}{}{}{}}
\newlabel{stab:cedar_vs_best_ml}{{5}{12}{}{}{}}
\newlabel{stab:fe_poc}{{6}{12}{}{}{}}
\newlabel{stab:refinement2}{{7}{13}{}{}{}}
\newlabel{stab:error_taxonomy}{{8}{13}{}{}{}}
\newlabel{stab:refinement}{{9}{14}{}{}{}}
\newlabel{stab:mimic}{{10}{15}{}{}{}}
\newlabel{stab:ablation}{{11}{16}{}{}{}}
\newlabel{stab:feature_summary}{{12}{17}{}{}{}}
\newlabel{stab:collinear}{{13}{17}{}{}{}}
\newlabel{stab:s0_snippets}{{14}{18}{}{}{}}
\newlabel{stab:s0_snippets_t1d}{{15}{19}{}{}{}}
\newlabel{stab:cedar_vs_vanilla}{{16}{20}{}{}{}}
\newlabel{stab:sample_sizes}{{17}{20}{}{}{}}
\newlabel{sfig:backbone_vs_ml}{{1}{23}{}{}{}}
\newlabel{sfig:economics}{{2}{24}{}{}{}}
\newlabel{sfig:annotation}{{3}{25}{}{}{}}
\newlabel{sfig:omitted_configs}{{4}{26}{}{}{}}
\newlabel{sfig:faithfulness}{{5}{27}{}{}{}}
\newlabel{sfig:error_analysis}{{6}{28}{}{}{}}
\newlabel{sfig:hybrid_b}{{7}{29}{}{}{}}
\newlabel{sfig:routing_policy}{{8}{30}{}{}{}}
\newlabel{sfig:cedar_refinement}{{9}{31}{}{}{}}
\newlabel{sfig:calibration}{{10}{32}{}{}{}}
\newlabel{sfig:regime}{{11}{33}{}{}{}}
\newlabel{sfig:modality}{{12}{34}{}{}{}}
\newlabel{sfig:temporal_val}{{13}{35}{}{}{}}
\newlabel{sfig:ablation_all}{{14}{36}{}{}{}}
\newlabel{sfig:prevalence}{{15}{36}{}{}{}}
\makeatother
